# Supplementary material for: An Adaptive Resample-Move Algorithm for Estimating Normalizing Constants
Source: arXiv:1604.01972 source file (2016-08-15)
Supplement: Supplementary file 1 [file appendixrbm.tex]

%!TEX root = main.tex

\section{Restricted Boltzmann Machines}\label{app:rbm}

\todo{[ some intro needed ]}

%\subsection{Computational Complexity}

The algorithm presented in \cite{AISmoments} is computationally very expensive: first the moments of the target distributions are estimated using 1000 independent Gibbs chains with 11000 Gibbs steps each, then the parameters of 9 intermediate RBMs have to be fit in order to match the averaged moments at 9 different temperatures (knots of a spline), and finally a geometric path with 10000 intermediate distributions is used in order to pass from one RBM at one knot to the next one, giving therefore 100000 intermediate distributions in total.

We can get an insight on how much faster ARM can be just evaluating the overall computational complexity of the Gibbs sampler used in the move-step, as this is the most time consuming operation both for ARM and AIS. Despite being not completely accurate, this comparison has the advantage of not depending on the efficiency of the implementation.
We can start by noticing that one particle of the ARM essentially corresponds
to one run of AIS. At iteration $n$ of ARM the Gibbs sampler has complexity $\mathcal{O}(tHn)$, where $t$ is the number of Gibbs steps used. As $n=1,\ldots,N$, the overall complexity is $\mathcal{O}(tHN(N+1)/2)$.
For AIS (both using geometric and moment averages) on the other hand, given $K$ intermediate distributions, the complexity is $\mathcal{O}(tHNK)$. 
To get estimates accurate enough we have $t(N+1)/2 \ll K$: with the numbers used to obtain Figure \ref{fig:rbm_res} for example, we have $3925 \ll 100000$. 

A part from this operation, AIS (MA) has other computationally expensive parts, such as the moment estimation of the target distribution and the moment matching.
